# Supplementary material for: Sensing viruses by mechanical tension of DNA in responsive hydrogels
Source: arXiv:1310.5531 source file (2013-10-21)
Supplement: Supplementary file 1 [file supp.pdf]

# Supplementary Material: Sensing viruses by mechanical tension of DNA in responsive hydrogels

Jaeoh Shin,[1] Andrey G. Cherstvy,[1] and Ralf Metzler[1,2]

[1] *Institute for Physics & Astronomy, University of Potsdam, D-14476 Potsdam-Golm, Germany*
[2] *Department of Physics, Tampere University of Technology, FI-33101 Tampere, Finland*

In this Supplementary Material we present details of the analysis of the simulations data and show additional Figures to clarify some details mentioned in the main text.

We also checked that for a fixed DNA-DNA separation, rather than a fixed DNA-surface distance $z_0$, the system behavior remains qualitatively similar for varying virus size, including the scaling relation, Eq. (7). The $\theta(\epsilon_A)$ values reveal however somewhat larger changes for different $R$ values. In this case, not only the curvature of the surface and the number of available sites for the DNA adsorption varies as $R$ increases, but also the DNA-capsid distance decreases. This causes the DNA adsorption to proceed easier and the corresponding $\theta$ values to increase somewhat at larger $R$ values, see Fig. S1.

The results presented in Fig. S2 support our assumption to upscale the effect of a single DNA to the case when several DNA chains surround a virus. Namely, for a typical shell radius used in the simulations, $R = 6\sigma$, and for the coverage fraction $p = 1/3$ the number of attractive sites on the shell is $\approx 260$. For a typical ssDNA length of $n$ =101 bases the number of bound monomers is <60. Thus, for two ssDNAs binding to each viral particle the fragments of adsorbed DNA have sufficient freedom to rearrange themselves on the shell surface, and their contribution to the gel contraction is additive.

For strong DNA-virus attraction ($\epsilon_A \gtrsim 3$) the length of ssDNA increases considerably, and it is sometimes problematic to extract $l_{ss}^{opt}$ from the simulations. Physically, this situation corresponds to nearly completely molten DNA, as one can anticipate for this case of highly preferential ssDNA-shell adsorption. Here, it is necessary to account for the above-mentioned geometric factor $C$, the fraction of active surface monomers $p$, and, most importantly, for the fact that a polymer segment can bind to several monomers on the sphere surface at once (according to the used adsorption criterion). This alters the slope of $f(\epsilon_A)$ shown in Fig. 7. In simulations, the contraction force was also obtained using the WHAM method.

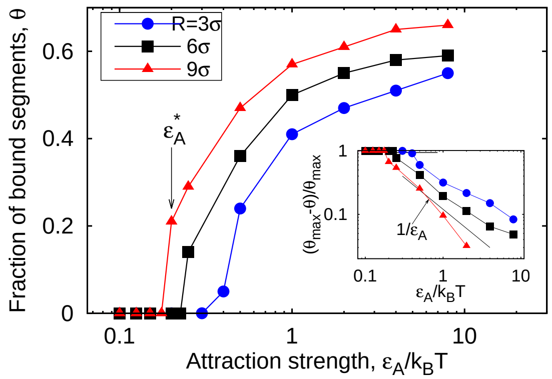


Figure S1: The same as in Fig. 3, but for a constant DNA-DNA separation, $s = 28\sigma$. The DNA-shell separation $z_0$ changes with $R$ according to $s/2 = z_0 + R$. The inset shows the residual fraction of non-adsorbed monomers that scales as $1/\epsilon_A$. Other parameters are the same as in Fig. 3.

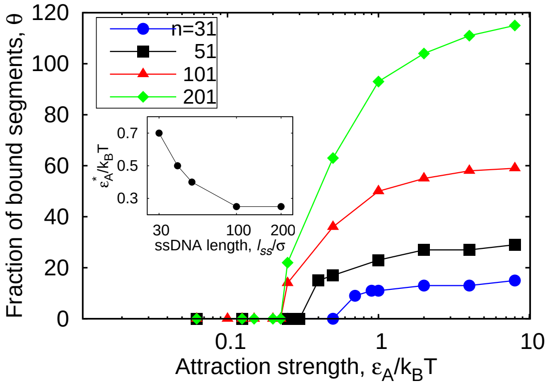


Figure S2: The effect of polymer length on the sharpness of ssDNA-shell adsorption transition. The parameters are the same as in Fig. 3, and $R = 6\sigma$.

We compute the pulling force on the ends of dsDNA due to the presence of partially adsorbed melted ssDNA strands as follows. After determining the optimal length of the ssDNA, $l_{ss}^{opt}$, we vary the DNA end-to-end distance, $y_0$. This alters the length of ssDNA potentially available for adsorption onto the capsid surface. The latter is subject to a parabolic biasing potential in the WHAM method, $k_w(y - y_0)^2/2$. This enables us to enumerate the probability density function for the chain ends, $p(y)$. Subtracting this parabolic potential from the restored free energy of the system, $U(y) = -k_BT \log[p(y)] - k_w(y-y_0)^2/2$, we obtain that for positions close to $y = y_0$ we get a linear dependence for the DNA-virus attraction energy on $y_0$, namely $U(y_0) \approx fy_0$. The proportionality factor is the contraction force $f$ acting on the DNA ends.

Finally, Eq. (6) couples the material parameters to the relative contraction of the DNA ends, $\delta l/l_{ss}^{opt}$. In this expression, the optimal ssDNA length is used (see Fig. S3), that is found self-consistently for each value

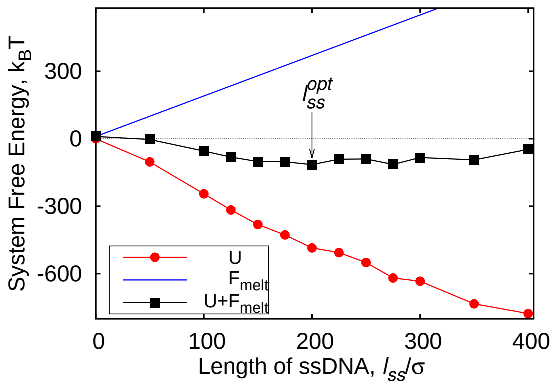


Figure S3: Total free energy of partially molten DNA as function of the number of ssDNA monomers. Parameters: $R = 6\sigma$, $z_0 = 8\sigma$, $\epsilon_A = 2.2k_BT$, $p = 1/3$, $F_s = 10k_BT$, and $\Delta F = 0.3k_BT$.

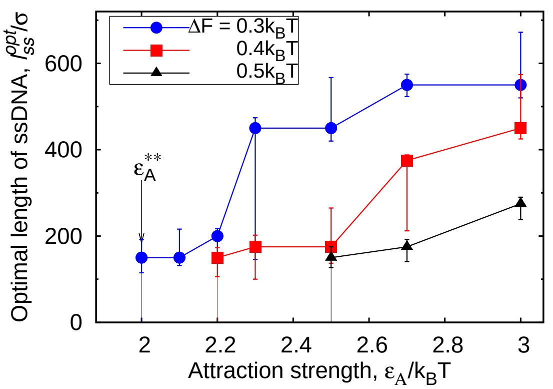


Figure S4: The optimal length of ssDNA grows with virus-DNA attraction strength $\epsilon_A$. The error bars reflects the degree of fluctuations of adsorbed ssDNA monomers. Parameters are the same as in Fig. S3.

of ssDNA-virus attraction strength, $\epsilon_A$. Clearly, for stronger ssDNA-virus attractions progressively longer stretches of ssDNA get adsorbed to the viral shell, yielding larger contraction forces $f$, see Fig. S4 and Fig. 7. The proportionality constant $C$ in Eq. (1) and Fig. 7 varies if one uses a constant length of ssDNA when computing the relative gel contraction. This constant accounts for the fact that a single chain monomer can simultaneously bind several attractive sites on the capsid surface (thus $C$ decreases as fraction $p$ decreases).

The error bars shown in Fig S4 are for different depths of the free energy wells and their profile. The procedure to determine these error bars is as follows. After obtaining the ssDNA length $l_{\rm ss}^{\rm opt}$ in the overall minimum of the free energy functional, we are interested in how far thermal fluctuations can alter the position of this minimum. We fix the value of the allowed thermal jiggling to $k_BT/5$ per adsorbed bead of the ssDNA and compute from the shape of the free energy function what the allowed changes $l_{\rm ss}^{\rm opt}$ are such that we remain within these free energy thresholds. For shallow free energy wells large fluctuations in the adsorbed ssDNA length are possible, such that the size of the corresponding error bars is large. Due to an asymmetric shape near the free energy minimum the fluctuations with the same tolerance yield different deviations in the length of adsorbed ssDNA to either side of the minimum. This effect gives rise to asymmetric error bars in the graphs. From these error bars one can also compute the restoring force towards the free global energy minimum acting on the system.
